# Supplementary material for: Optimal Control for Linear Networked Control Systems with Information Transmission Constraints
Source: arXiv:2109.10666 source file (2021-09-22)
Supplement: Supplementary file 1 [file appendix_redundant_controls.tex]

\section{Redundant Controls}

Intuitively, if the information available to the controller is very little (i.e. the measurement budget $N_m$ is very low), then using more control actions can do very little to help solve the problem (i.e. using large $N_c$). To justify this intuition, we discuss a simplified problem and an observed property about it.

\subsection{Intuition from a sample problem}

Consider the following simplified problem and its solutions.

\begin{problem}
    \label{prob:redundant_controls1}
    Assume that there is a measurement schedule $\modeSymbol^m$ defined as:
    $$
    \sigma^m_t =
    \begin{cases}
        1 & t = 0, \\
        1 & t = T, \\
        0 & \text{otherwise}
    \end{cases}
    $$
    % \begin{itemize}
    %     \item $\sigma^m_0 = 1$
    %     \item $\sigma^m_t = 0, \quad \forall t \in [1,T-1]$
    %     \item $\sigma^m_T = 1$
    % \end{itemize}
    and that there is a control schedule $\modeSymbol^c$ defined with only two nonzero times $t_1,t_2 \in [0,T-1]$ such that
    $$
        \sigma^c_t =
        \begin{cases}
            1 & t \in \{t_1,t_2 \}\\
            0 & \text{otherwise}.
        \end{cases}
    $$
    Determine whether or not there exists a control schedule with only one nonzero control time such that \emph{the system reaches the same state at time $T$} (i.e. $x_T$ is the same for the controller with $\modeSymbol^m$ and $\modeSymbol^c$ as it is for $\modeSymbol^m$ and $(\modeSymbol^c)'$ where $(\modeSymbol^c)'$ has only one nonzero control time.)
\end{problem}

% \begin{problem}
%     Consider the optimal solution $(\mathcal{T}_C^*,u^*)$ to the simplified problem with constraint $|\mathcal{T}_C| \geq 2$ and the optimal solution $(\mathcal{T}_C',u')$ to the simplified problem with constraint $|\mathcal{T}_C|=1$. Prove whether or not the objective value of $(\mathcal{T}_C^*,u^*)$ is $\eta_x^*$ and the objective value of $(\mathcal{T}_C',u')$ is $\eta_x'$, then the objective values are equal.
% \end{problem}

% \begin{lemma}
%     Consider the optimal solution $(\mathcal{T}_C^*,u^*)$ to the simplified problem with constraint $|\mathcal{T}_C| \geq 2$ and the optimal solution $(\mathcal{T}_C',u')$ to the simplified problem with constraint $|\mathcal{T}_C|=1$. If the objective value of $(\mathcal{T}_C^*,u^*)$ is $\eta_x^*$ and the objective value of $(\mathcal{T}_C',u')$ is $\eta_x'$, then the objective values are equal.
% \end{lemma}

\begin{proposition}
    For any system, there always exists a control schedule with only one nonzero control time that satisfies the condition of Problem \ref{prob:redundant_controls1}.
\end{proposition}

\begin{proof}
    Consider the following components of the solutions: $\mathcal{T}_C = \{ t_1,t_2 \}$ and $\mathcal{T}_C^* = \{ t_1^* \}$.
    
    Without loss of generality and for ease of exposition, we consider the system \eqref{eq:system_w_missing_meas} without noise. Consider the following equations for the trajectory of the solution to the problem with $\mathcal{T}_C$ under such a system:
    $$
    \begin{array}{rll}
      x_t & = A^t x_0 & t < t_1 \\
      x_{t+1} & = A^t x_0 + \sum_{\tau=t_1}^t A^{t-\tau} B u_{t_1} & t_1 \leq t < t_2 \\
      x_{t+1} & = A^t x_0 + \sum_{\tau=t_1}^t A^{t-\tau} B u_{t_1} + \sum_{\tau=t_2}^t A^{t-\tau} B u_{t_2} & t_2 \leq t < T 
    \end{array}
    $$
    
    We are interested in the final state of the system $x_T$. Which can be written as follows:
    
    % $$
    % \begin{array}{rl}
    %     x_t = & A^t x_0 + \cdots \\
    %      & \left[
    %         \sum_{\tau=\tau_1}^t A^{t-\tau} B F^{(1)}_{\tau_1^*,0} + \sum_{\tau=\tau_2}^t A^{t-\tau} B F^{(2)}_{\tau_2^*,0}
    %         \right] y_0 + \cdots \\
    %      & \left[
    %         \sum_{\tau=\tau_1}^t A^{t-\tau} B f^{(1)}_{\tau_1^*} + \sum_{\tau=\tau_2}^t A^{t-\tau} B f^{(2)}_{\tau_2^*}
    %         \right]
    % \end{array}
    % $$
    
    % Which can be rewritten as follows:
    $$
    \begin{array}{rl}
        x_T = & A^{T-1} x_0 + \cdots \\
         & \left[
            \sum_{\tau=t_1}^{t_2-1} A^{t-\tau} B F^{(1)}_{t_1,0} + \sum_{\tau=t_2}^t A^{t-\tau} B (F^{(2)}_{t_2,0} + F^{(1)}_{t_1,0})
            \right] y_0 + \cdots \\
         & \left[
            \sum_{\tau=t_1}^{t_2-1} A^{t-\tau} B f^{(1)}_{t_1} + \sum_{\tau=t_2}^t A^{t-\tau} B (f^{(2)}_{t_2} + f^{(1)}_{t_1})
            \right]
    \end{array}
    $$
    
    From this definition, it is clear that by choosing $t_1^* = t_1$ and letting the gains $\{ F^*_{t,\tau} , f^*_\tau \}$ be determined by the summations above the exact same point may be reached by linear gains as shown in the equation below:
    $$
    x_{t+1} = A^t x_0 + \sum_{\tau=\tau_1}^t A^{t-\tau} B ( F_{\tau,0}^* y_0 + f_{t_\tau}^*) .
    $$
    Thus, it should be possible to choose a schedule $\mathcal{T}_C^*$ such that a control sequence exists which leads to the same final point $x_T$ as the schedule $\mathcal{T}_C$.
\end{proof}

While this property does indicate that controls can be redundant, it is hard to use it to prove redundancy for the specific problems of this paper (Problem \ref{prob:control_asap} and \ref{prob:control_alap}). We would like to analyze the safety of entire trajectories and not just the final state. A problem that would be more appropriate would be:

\begin{problem}
    \label{prob:redundant_controls2}
    Assume that there is a measurement schedule $\modeSymbol^m$ defined as:
    $$
    \sigma^m_t =
    \begin{cases}
        1 & t = 0, \\
        1 & t = T, \\
        0 & \text{otherwise}
    \end{cases}
    $$
    % \begin{itemize}
    %     \item $\sigma^m_0 = 1$
    %     \item $\sigma^m_t = 0, \quad \forall t \in [1,T-1]$
    %     \item $\sigma^m_T = 1$
    % \end{itemize}
    and that there is a control schedule $\modeSymbol^c$ defined with only two nonzero times $t_1,t_2 \in [0,T-1]$ such that
    $$
        \sigma^c_t =
        \begin{cases}
            1 & t \in \{t_1,t_2 \}\\
            0 & \text{otherwise}.
        \end{cases}
    $$
    Determine whether or not there exists a control schedule with only one nonzero control time such that \emph{the system reaches the same state at all times $t \in [0,T]$} (i.e. $x_t$ is the same for the controller with $\modeSymbol^m$ and $\modeSymbol^c$ as it is for $\modeSymbol^m$ and $(\modeSymbol^c)'$ where $(\modeSymbol^c)'$ has only one nonzero control time.)
\end{problem}

\begin{proposition}
    There exist systems for which a control schedule with only one nonzero control time cannot satisfy the condition of Problem \ref{prob:redundant_controls2}.
\end{proposition}

\begin{proof}
    A property which would 
\end{proof}

This property can be used to show that having two control times with no measurement time in between is redundant.  In general this means that a solution with $|\mathcal{T}_C| \leq |\mathcal{T}_M|+1$ can achieve the same objective value as one with $|\mathcal{T}_C| > |\mathcal{T}_M|+1$.

% \AA{Very interesting ! It looks great :-) Do we need to assume that $B$ is full rank ? I think so because if not, we can't control all modes of the system with only one control. For example, if $A=\begin{bmatrix}0&2\\ 3& 0\end{bmatrix}$, $B=[1\; 0]^\top$ and $C=\begin{bmatrix}1&0\\ 0&1 \end{bmatrix}$, $v(t)\approx 0$. With such an example, we know exactly the state but need two controls to set the state to the origin.}

% \KR{This is the correct reasoning. We need a condition on whether or not the controllability matrix is full rank.}

Throughout the proof we will make the following assumption
\begin{assumption}
    There exists a single point in time $t^*$ where $\|x_c(t^*)\|= \eta_x^*$ and there exists a single point in time $t'$ where $\|x_c(t')\|=\eta_x'$.
\end{assumption}
