# Supplementary material for: Optimal Control for Linear Networked Control Systems with Information Transmission Constraints
Source: arXiv:2109.10666 source file (2021-09-22)
Supplement: Supplementary file 2 [file solution_properties.tex]

\section{Properties of the Solution} \label{subsec:properties}

\KR{A polytope $\mathcal{P} \subseteq \R^{n}$ is \emph{full-dimensional} if there exists an element $p\in\mathcal{P}$ and a radius $r>0$ such that $\{ x \in \R^n \; | \; \| p - x \| \leq r \} \subseteq \mathcal{P}$.}

There were many possible constraints considered and solution methods proposed for Problem \ref{prob:control_asap}. In this section, we analyze some of those proposals and discuss the reasoning behind why they could be considered and what advantages they provide in the synthesis for problems like Problem \ref{prob:control_asap}.

\subsubsection{Constraints on the Measurement Signal $\modeSymbol^m$}

The property of observability (or detectability) of a system is one of the fundamental constraints which determines the feasibility of Problem \ref{prob:control_asap} (similarly, observability determines the objective value of \ref{prob:control_alap}). In the measurement scheduling problem, this property can be analyzed using the methods of \cite{jungers2018observability}. An observability matrix can be defined for the system in \ref{eq:system_w_missing_meas} as follows:

\begin{definition}[Observability Matrix $\mathcal{O}_{\sigma^m}$ \cite{jungers2018observability}]
    Given a measurement signal $\modeSymbol^m$, the \emph{observability matrix} of the system \eqref{eq:system_w_missing_meas} at time $t$ is:
    \begin{equation*}
        \mathcal{O}_{\sigma^m}(t) =
        \begin{bmatrix}
            \modeSymbol^m_0 C \\
            \modeSymbol^m_1 CA \\
            \vdots \\
            \modeSymbol^m_{t-1} CA^{t-1}
        \end{bmatrix}\in \mathbb{R}^{(t+1)n_y \times n_x}.
    \end{equation*}
\end{definition}

The null space of this matrix can be analagously called the unobservable space of initial conditions for system \eqref{eq:system_w_missing_meas} when no noise is present. Intuitively, the choice of measurement times is determining the unobservable initial conditions of the system and should somehow incorporate information about which initial conditions may violate our constraints on the output $z_t$.

Now, consider the set of initial conditions which \emph{escape} the performance constraint at time $T$:
$$
\EscapeSetFromXatT =
\left \{
    x_0 \in \mathcal{X}_0 
    \; | \;
    \exists \{ w_\tau \}_{\tau=0}^{T-1} \text{ s.t. } z_T^{(ol)} \notin \performanceSet
\right \}.
$$
where the open loop performance output at time $T$, $z_T^{(ol)}= D ( A^{T} x_0)+d$, is a linear function of $x_0$. The variable $z_T^{(ol)}$ can also be redefined as $z_T^{(ol)}= D ( A^{T} x_0 + \sum_{\tau=0}^{T-1} A^{T-1-\tau} w_\tau)+d$ with $w_\tau$ being parallel to $x_0$, but we omit this more general definition for clarity of the exposition.

A relationship between $\mathcal{O}_{\sigma^m}(T)$ and $\EscapeSetFromXatT$ can then be used to define an overapproximation of the feasible set of solutions to Problem \ref{prob:control_asap}:

\begin{proposition}
    \label{prop:observability_of_optimal_sigma}
    Consider the safety problem (Problem \ref{prob:control_asap}) with sets $\mathcal{W},\V,\performanceSet$ being symmetric about the origin and $d=0$ along with the set $\EscapeSetFromXatT$ with respect to the dynamics in \ref{eq:system_w_missing_meas}. The problem is feasible for $ T^* \geq T$ only if there exists a measurement signal $\sigma^m \in \zeroOneSet^{T}$ such that
    $$
    \EscapeSetFromXatT 
    \cap
    \mathcal{N}( \mathcal{O}_{\sigma^m}(T) )
    = \emptyset.
    $$
\end{proposition}
% \begin{proof}
%     Suppose that for any arbitrary choice of $\modeSymbol^m$, there exists an initial state 
%     $x_0^* \in
%     \tilde{\mathcal{X}}_0(T) 
%     \cap
%     \mathcal{N}( \mathcal{O}_{\sigma^m}(T) )
%     $.
%     By symmetry, this implies that  $-x_0^* \in \tilde{\mathcal{X}}_0(T)$ and $DA^Tx_0, -DA^T x_0 \notin \performanceSet.$ Then, by expanding the closed loop performance output when the disturbances are zero (e.g. $w=0,v=0$ for all $t$) one obtains
%     $$ 
%     z_T = D A^T x_0 + D \sum_{\tau = 0}^{T-1} A^{T-1-\tau} B f_\tau.
%     $$
%     The open loop controller $f_\tau=0$ and $f_{T-1} = s - D A^T x_0$ where $s \in \performanceSet$ can guarantee that $z_T \in \performanceSet$, but note that for the initial condition $-x_0$, $z_T = -2D A^T x_0 + s \notin \performanceSet$. In fact, for any open loop controller which cannot distinguish between $x_0$ and $-x_0$, we can show that one of the initial conditions will violate $z_T \in \performanceSet$.
    
%     Thus, if one cannot find a $\sigma^m$ such that $\tilde{\mathcal{X}}_0(T) \cap \mathcal{N}( \mathcal{O}_{\sigma^m}(T) )$ is empty, then there will exist an initial condition for which no open loop control can guarantee the performance variable at time $T$, $z_T$, remains within the symmetric safe set $\performanceSet$.
% \end{proof}

The proposition can be extended by considering a different definition of $\EscapeSetFromXat{T^*}$ where $z_T^{(ol)}$ is redefined as $z_T^{(ol)}= D ( A^{T} x_0 + \sum_{\tau=0}^{T-1} A^{T-1-\tau} w_\tau)+d$ with $w_\tau$ being parallel to $x_0$. % By translating $\performanceSet$, we can assume $d=0$ wlog. Is this still possible?

Proposition \ref{prop:observability_of_optimal_sigma} leads to the following corollary:
\begin{corollary}
    \label{cor:meas_schedule_feasible_set}
    For a given Problem \ref{prob:control_asap}, let $T^*$ and $(\sigma^m)^*$ be the optimal solutions of the problem and $T_1$ be the smallest time such that $\EscapeSetFromXat{T_1}$ is full dimensional. If $T_1$ exists and $T_1 \leq T^*$, then $\mathcal{O}_{(\sigma^m)^*}(T_1)$ has full rank (i.e. the system without noise is observable at time $T_1$).
\end{corollary}

This corollary explains that the solution of Problem \ref{prob:control_asap} will contain an initially observable measurement schedule, if there are enough measurements available in the budget. By applying this argument recursively, this corollary can be extended to say that all nontrivial measurement schedules must contain observable prefixes. Crucially, this corollary explains that all optimal schedules should contain an observable prefix and that adding such a constraint would reduce the search space and reduce the computation time of the solution.

\subsection{Proof of Proposition \ref{prop:observability_of_optimal_sigma}}

Suppose that for any arbitrary choice of $\modeSymbol$, there exists an initial state 
$x_0^* \in
\tilde{\mathcal{X}}_0(T) 
\cap
\mathcal{N}( \mathcal{O}_{\sigma}(T) )
$.
By symmetry, this implies that  $-x_0^* \in \tilde{\mathcal{X}}_0(T)$ and $DA^Tx_0, -DA^T x_0 \notin \performanceSet.$ Then, by expanding the closed loop performance output when the disturbances are zero (e.g. $w=0,v=0$ for all $t$) one obtains
$$ 
z_T = D A^T x_0 + D \sum_{\tau = 0}^{T-1} A^{T-1-\tau} B f_\tau.
$$
The open loop controller $f_\tau=0$ and $f_{T-1} = s - D A^T x_0$ where $s \in \performanceSet$ can guarantee that $z_T \in \performanceSet$, but note that for the initial condition $-x_0$, $z_T = -2D A^T x_0 + s \notin \performanceSet$. In fact, for any open loop controller which cannot distinguish between $x_0$ and $-x_0$, we can show that one of the initial conditions will violate $z_T \in \performanceSet$.

Thus, if one cannot find a $\sigma$ such that $\tilde{\mathcal{X}}_0(T) \cap \mathcal{N}( \mathcal{O}_{\sigma}(T) )$ is empty, then there will exist an initial condition for which no open loop control can guarantee the performance variable at time $T$, $z_T$, remains within the symmetric safe set $\performanceSet$.

\subsubsection{Constraints on the Control Signal $\modeSymbol^c$}

\subsubsection{Discrete Optimality}
